# Supplementary material for: A Review of Machine Learning for Cavitation Intensity Recognition in Complex Industrial Systems
Source: arXiv:2511.15497 source file (2025-12-15)
Supplement: Supplementary file 1 [file appendix.tex]

\setcounter{table}{0}
\setcounter{figure}{0}
\setcounter{equation}{0}
\setcounter{section}{0}
\setcounter{subsection}{0}

\section{Definition of cavitation}
\label{sec: cavitation knowledge}
Some standard knowledge about the physical phenomenon of cavitation which helps the cavitation data collection. Figure \ref{fig: civitation knowledge} illustrates how the local pressure changes in one dimensional flow. The valve would operate normally on cavitation-free status when the minimum pressure ${p}_{min}$ is higher than the vapor pressure ${p}_{v}$. In the case where ${p}_{v}>{p}_{min}$ cavitation begins. It is of great importance for valve manufacturers to know the minimum pressure of their valves. But, according to SAMSON AG, it can not be directly measured, since the minimum pressure occurs downstream of the constraint. In practice the cavitation coefficient ${x}_{FZ}$ has proven to give empirical guidance, which equals the ratio of the external pressure difference to the internal pressure difference. It can be determined empirically, by assuming that the cavitation noise begins only when minimum pressure ${p}_{min}$ equals vapor pressure ${p}_{v}$. Hence, the cavitation coefficient ${x}_{FZ}$ can be measured by the noise, which depends on the load of the valve. The equations of cavitation coefficient ${x}_{FZ}$ and operating pressure ratio ${x}_{F}$ are presented below:
\begin{equation}
{x}_{FZ}=\frac{{p}_{1}-{p}_{2}}{{p}_{1}-{p}_{min}}
\end{equation}
\begin{equation}
{x}_{F}=\frac{{p}_{1}-{p}_{2}}{{p}_{1}-{p}_{v}}
\end{equation}
where ${p}_{1}$ is the inlet pressure, ${p}_{2}$ is the outlet pressure, ${p}_{min}$ is the minimum pressure in the valve and ${p}_{v}$ is the vapor pressure. When all coefficients are known over the full opening range of the valve, the following statements can be made.
\begin{itemize}
\item ${x}_{F}<{x}_{FZ}$: The valve operates without cavitation. The Flow is merely turbulent or laminar.
\item ${x}_{F}\geq {x}_{FZ}$: For ${x}_{F}={x}_{FZ}$, the valve operates with incipient cavitation. As the difference between ${x}_{FZ}$ and ${x}_{F}$ increases, the cavitation zone grows because the pressure drops as a result of increasing flow velocities.
\item ${x}_{F}>1$: Here the bubbles do not implode in the valve but rather continue to flow into the pipe, as the outlet pressure ${p}_{2}$ is lower than the vapor pressure. This phenomenon is known as flashing.
\end{itemize}
The cavitation coefficient ${x}_{FZ}$ should be as high as possible over the whole valve operation range, so that damage to the valve due to cavitation is minimized. A final remark: The cavitation coefficient ${x}_{FZ}$ only applies to the fluid, where it was empirically measured. Its valve vary for different liquid mediums, due to change in viscosity, content of dissolved gas \cite{oldenziel1979bubble} and so on \cite{kiesbauer2001control}.
\input{input_figs/input_appendix_knowledge}

\section{Examples of cavitation states}
\label{sec: examples of cavitation states}
Figures \ref{fig: state example dataset1}, \ref{fig: state example dataset2} and \ref{fig: state example dataset3} show examples of different cavitation states for Cavitation 2017, Cavitation 2018 and Cavitation 2018-noise, respectively.
\input{input_figs/input_appendix_example}

\section{Discrete Fourier transform}
\label{sec: Discrete Fourier transform}
\subsection{From continuous Fourier transform to discrete Fourier transform}
\noindent Discrete Fourier transforms (DFT) can be derived in many ways. Since the Fourier transform (FT) is originally designed for continuous signals. Therefore, we will derive the DFT from the one-dimensional continuous Fourier transform (CFT). Specifically, given a continuous time signal $f(t)$, 1D CFT is given by:
\begin{equation}
\label{eq: CFT}
F(u)=\int^{+\infty }_{-\infty }f(t){e}^{-2j\pi ut}dt
\end{equation}
The continuous function $f(t)$ is sampled once at a time interval $\Delta T$ from a certain time (noted as moment $0$) and a total of N times. Then, we get a discretised sequence:
\begin{equation}
\label{eq: discretised sequence1}
f(\Delta T),f(2\Delta T),\ldots ,f(N\Delta T)
\end{equation}
and the discrete sequence is denoted as:
\begin{equation}
\label{eq: discretised sequence2}
\hat{f}(0),\hat{f}(1),\ldots ,\hat{f}(N-1)
\end{equation}
where for the other unsampled points, i.e. $\forall t\notin \left \{\Delta T,\ldots ,N\Delta T\right \}$, the value of the function for these points are $0$, i.e. $f(t)=0$. Applying equations \ref{eq: CFT} and \ref{eq: discretised sequence1}, we have
\begin{small}
\begin{equation}
\begin{aligned}
F(u)&=\int^{+\infty}_{-\infty}f(t){e}^{-2j\pi ut}dt\\
&=\int^{0}_{-\infty}+\int^{N\Delta T}_{0}+\int^{+\infty}_{N\Delta T}f(t){e}^{-2j\pi ut}dt\\
&=\int^{0}_{-\infty}+\int^{+\infty}_{N\Delta T}f(t){e}^{-2j\pi ut}dt+\int^{N\Delta T}_{0}f(t){e}^{-2j\pi ut}dt\\
&=0+\int^{N\Delta T}_{0}f(t){e}^{-2j\pi ut}dt\\
&=\int^{N\Delta T}_{0}f(t){e}^{-2j\pi ut}dt\\
&=F'(u)
\end{aligned}
\end{equation}
\end{small}
Next, we divide the interval $\left [0,N\Delta T\right]$ equally into N parts, the $i$-th interval ${k}_{i}=\left [\left(i-1\right)\Delta T,i\Delta T\right],i=1,\ldots ,N$ and the length of each interval is $N$. Let the value of the function taking the right endpoint on each interval ${k}_{i}$ be $f(i\Delta T){e}^{-2j\pi u\cdot (i\Delta T)}$. Furthermore, we can convert $F'(u)$ to the Riemann sum form of $F''(u)$ as follows
\begin{small}
\begin{equation}
\begin{aligned}
F''(u) &= \sum\limits_{i = 1}^N {\left[f\left(i\Delta T\right){e^{ - 2j\pi u \cdot \left(i\Delta T\right)}}\right]}\cdot \Delta T \\
&=\sum_{n=0}^{N-1}\left [f\left( \left(n+1\right)\Delta T\right){e}^{-2j\pi u\cdot\left(n+1\right)\Delta T}\right]\cdot\Delta T\\
&=\sum_{n=0}^{N-1}\left [ \hat{f}\left(n\right){e}^{-2j\pi u\cdot \left(n+1\right)\Delta T}\right]\cdot\Delta T
\end{aligned}
\end{equation}
\end{small}
If we let the length between the start and end times of sampling be 1 time unit, i.e. $N\Delta T=1$, then we have:
\begin{equation}
F''(u) = \frac{1}{N}\sum\limits_{n = 0}^{N - 1} {\hat f(n){e^{ - 2j\pi u\frac{{n + 1}}{N}}}} ,u = 0,1, \ldots ,N - 1
\end{equation}
which is exactly the formulation of the DFT.

\subsection{The convolvational theorem}
\label{sec: convolvational theorem}
\noindent The convolution theorem is the main property of the Fourier transform. Specifically, the FT for the circular convolution of two discrete sequences is equivalent to the dot product of these two sequences in the frequency domain. Given two discrete sequences $x\left [n\right]$ (signals) and $h\left [n\right]$ (filters), both of length $N$, the circular convolution can be defined as:
\begin{equation}
w\left [n\right]={\left(h\ast x\right)}_{n}=\sum_{m=0}^{N-1}h\left [m\right]x\left[{\left(n-m\right)}_{mod \,N}\right]
\end{equation}
where $mod$ denotes modulo operation and $\ast$ is convolution symbol. Consider the DFT of $w[n]$, we have:
\begin{small}
\begin{equation}
\begin{aligned}
W[k] &= \sum\limits_{n = 0}^{N - 1} {\sum\limits_{m = 0}^{N - 2} {h[m]x[{{(n - m)}_{mod \,N}}]} } {e^{ - j(2\pi /N)kn}}\\
&= \sum\limits_{m = 0}^{N - 1} {h[m]} {e^{ - j(2\pi /N)km}}\sum\limits_{n = 0}^{N - 1} {x[{{(n - m)}_{mod \,N}}]} {e^{ - j(2\pi /N)k(n - m)}}\\
&= H[k](\sum\limits_{n = m}^{N - 1} {x[n - m]} {e^{ - j(2\pi /N)k(n - m)}} + \sum\limits_{n = 0}^{N - 1} {x[n - m + N]} {e^{ - j(2\pi /N)k(n - m)}})\\
&= H[k](\sum\limits_{n = 0}^{N - m - 1} {x[n]} {e^{ - j(2\pi /N)kn}} + \sum\limits_{n = N - m}^{N - 1} {x[n]} {e^{ - j(2\pi /N)kn}})\\
&= H[k]\sum\limits_{n = 0}^{N - 1} {x[n]{e^{ - j(2\pi /N)kn}}} \\
&= H[k]X[k]
\end{aligned}
\end{equation}
\end{small}
where $H[k]X[k]$ is the multiplication of the two sequences in the frequency domain.

\subsection{Property of conjugate symmetric}
\label{sec: Property of conjugate symmetric}
\noindent The conjugate symmetry property is one of the properties of the DFT. Given a signal $x[n]$, we have:
\begin{small}
\begin{equation}
X[N - k] = \sum\limits_{n = 0}^{N - 1} {x[n]{e^{ - j(2\pi /N)(N - k)n}} = } \sum\limits_{n = 0}^{N - 1} {x[n]{e^{j(2\pi /N)kn}}}  = {X^*}[k]
\end{equation}
\end{small}
In our GRLNet, we use this property to reduce learnable parameters and redundant computations.
